# Supplementary material for: Topo-Field: Topometric mapping with Brain-inspired Hierarchical Layout-Object-Position Fields
Source: arXiv:2406.05985 source file (2024-12-25)
Supplement: Supplementary file 1 [file appendix.tex]

\appendix
\section{Appendix}
% \section{Appendix / supplemental material}

\setcounter{figure}{0}
\subsection{Scene Partation Example}
The scene can be partitioned into different regions using walls as dividers and lines can be aligned to these walls. This is similar in most scenarios, making the annotation of scene regions a straightforward task as shown in Fig. \ref{fig:divide_scene}.

\begin{figure}[ht]
\centering
\includegraphics[width=0.6\linewidth]{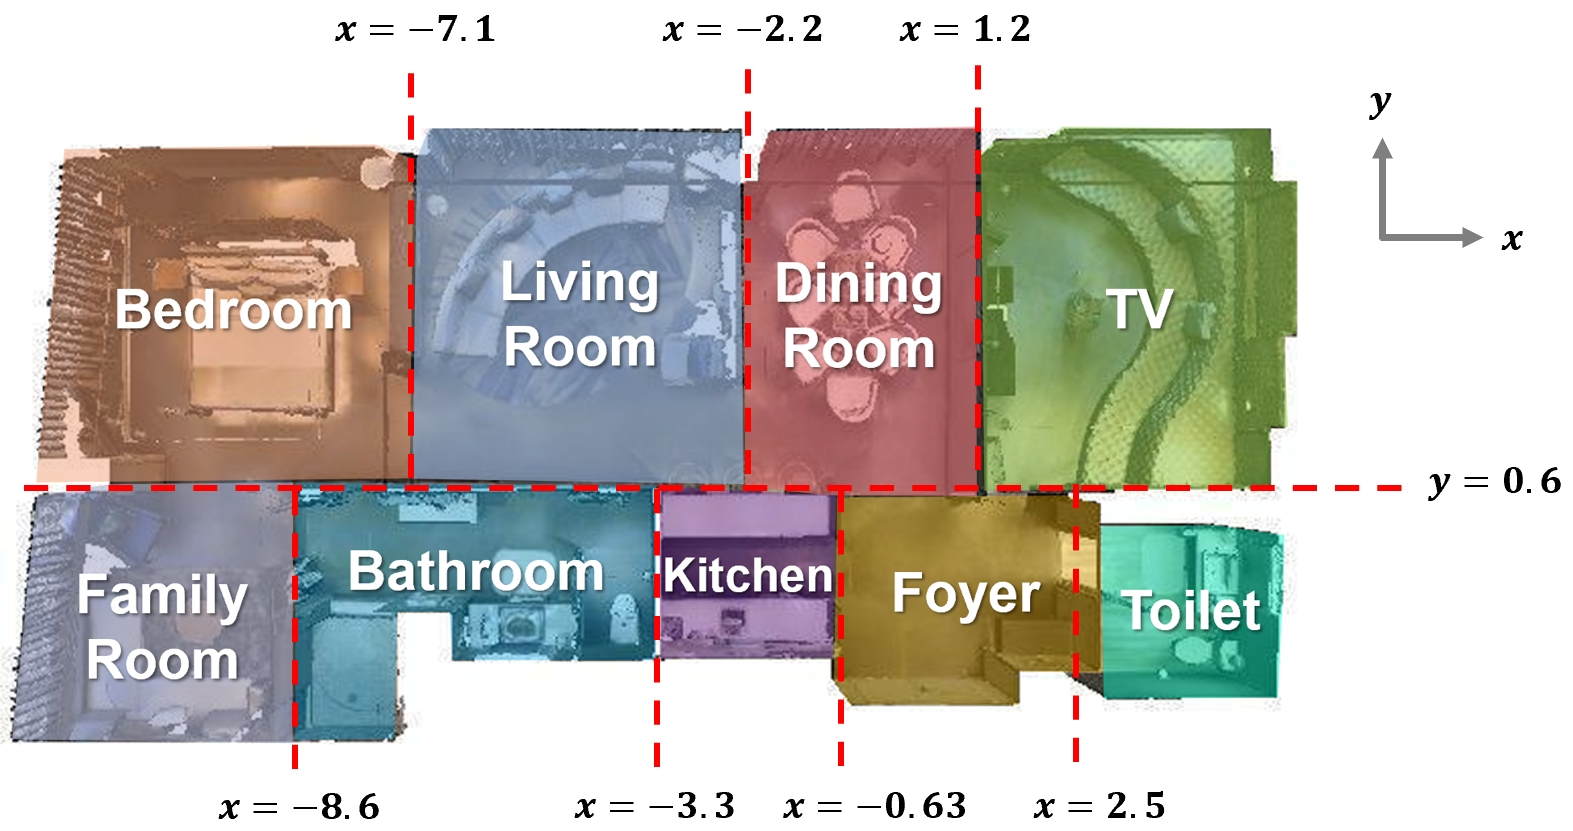}
\caption{Using walls as dividers to associate lines with them, the scene can be divided into various regions and 3D points can be labeled with related regions easily.}
\label{fig:divide_scene}
\end{figure}

% Optionally include supplemental material (complete proofs, additional experiments and plots) in appendix.
% All such materials \textbf{SHOULD be included in the main submission.}
\subsection{Vision-language Embeddings Similarity of Region and Objects}
To demonstrate that the relationship of the vision-language and semantic embeddings for different regions is related to our intuition, we compare the similarity in region-region and object-region form and show the results in Fig. \ref{fig:embed}. It can be seen that based on general knowledge, cognitively related regions (e.g., the dining room and kitchen) and object-region pairs (e.g., sink and kitchen) are also more correlated in the vision-language and semantic feature spaces.
\begin{figure}[ht]
\centering
\subfigure[]{
\begin{minipage}[b]{.9\linewidth}
\centering
\includegraphics[width=\linewidth]{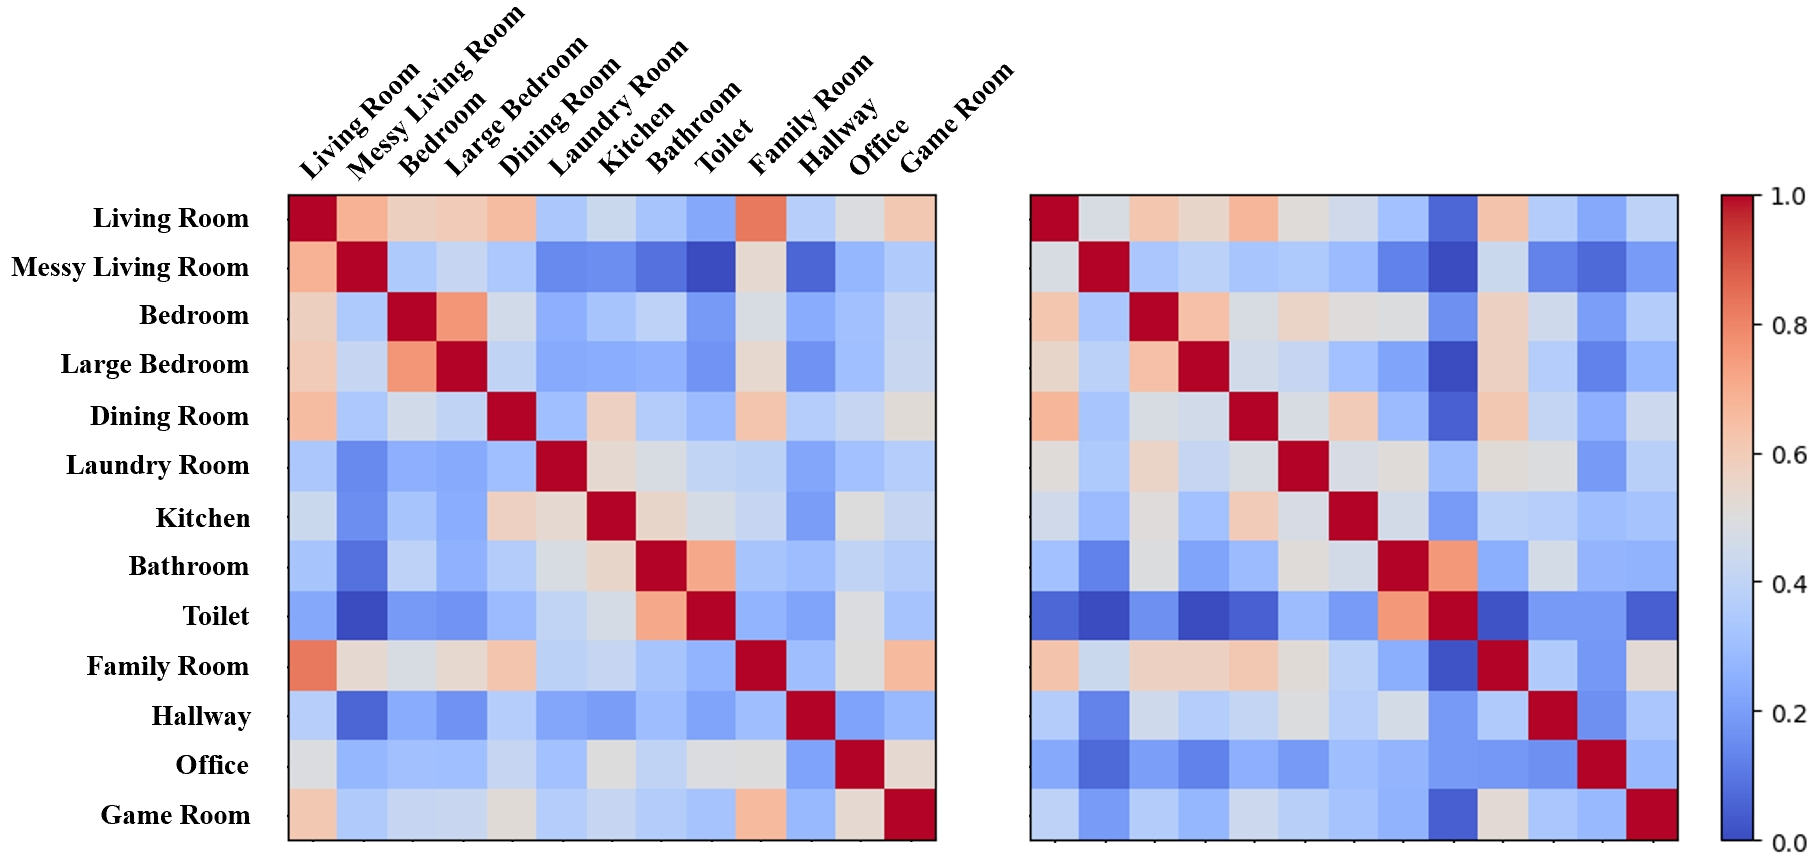}
\end{minipage}}
\subfigure[]{
\begin{minipage}[b]{.9\linewidth}
\centering
\includegraphics[width=\linewidth]{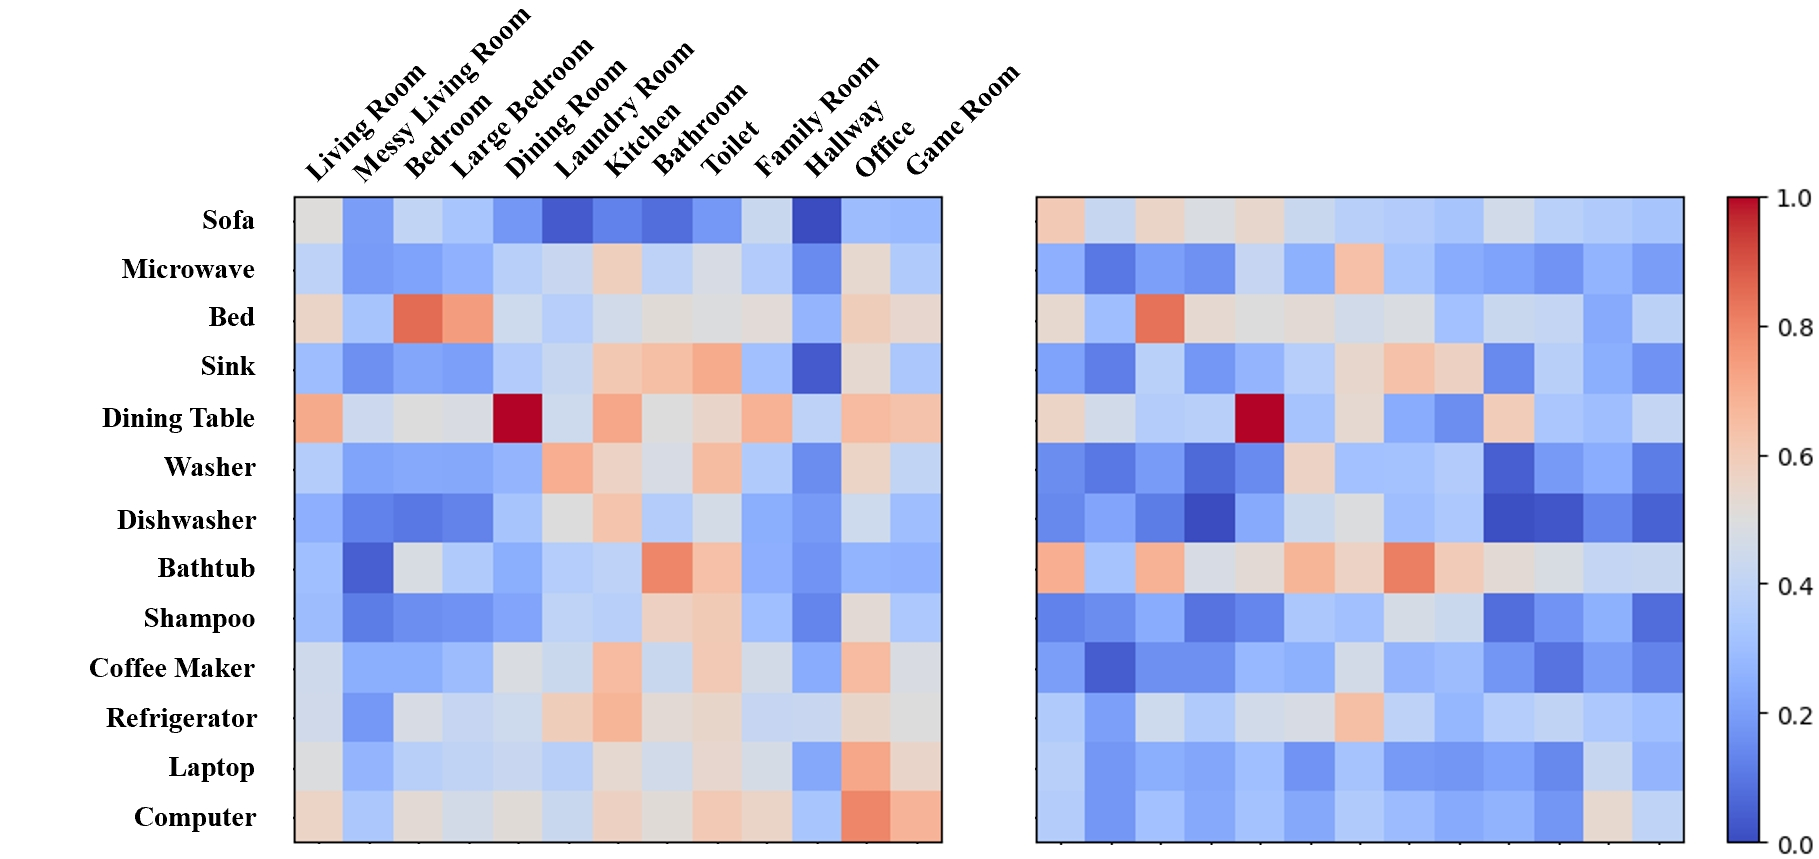}
\end{minipage}}
\caption{The similarity of a set of region embeddings (as shown in a) and object-region embeddings (as shown in b). The left graph shows the vision-language embedding similarity and the right one shows the semantic embedding similarity.}
\label{fig:embed}
\end{figure}

\subsection{Ablation Study}
To explicitly encode the region information, we apply the LVM to process the background pixels out of the object bounding box and LLM to encode the region label text. What's more, for object pixels, object label text is combined with the region text in the form of 'object in the region' before being encoded by LLM. To ablate the contribution of vision-language embeddings from CLIP and semantic embeddings from Sentence-BERT in encoding region features, we compare different weight settings between the v-s embeddings when inferring the regions with 3D position inputs. Results are shown in Fig. \ref{fig:ablation2}. It can be seen that both vision-language embeddings and semantic embeddings are indispensable, and weight settings with the greatest results are used for Topo-Field.

% \textbf{Source of Region Information.} In our very initial version, we assume that objects with region text include enough information to encode region layouts rather than encoding the background appearance. The region embeddings completely come from the region text label, and object embeddings are learned separately. Fig. \ref{fig:exp_ablation} shows the difference in embedding processing between the initial version and the current method. Ablation results in Fig. \ref{fig:ablation2} show that context and layout information in background pixels is necessary for layout-object-position association.

% \begin{figure}[p]
% \centering
% \subfigure[]{
% \includegraphics[width=0.5\linewidth]{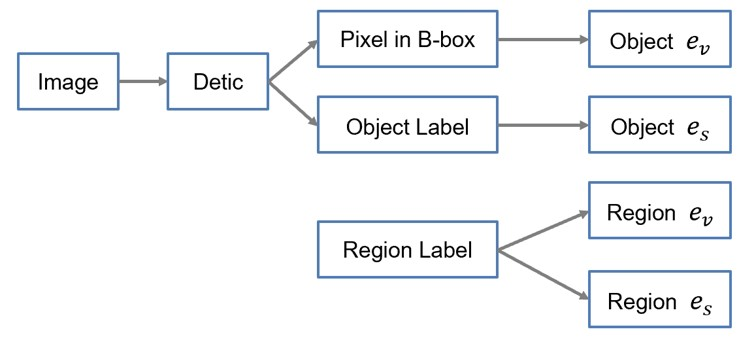}}
% \subfigure[]{
% \includegraphics[width=0.5\linewidth]{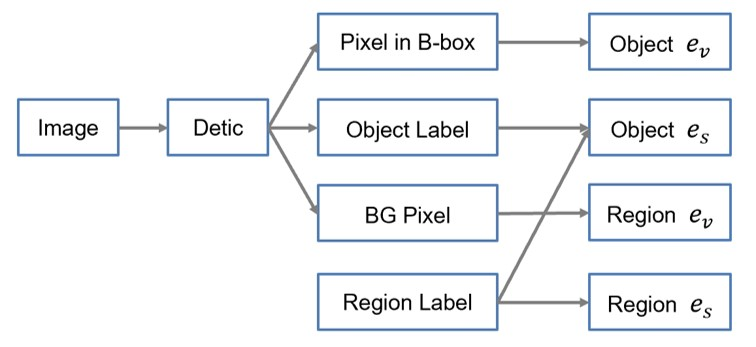}}
% \caption{The different source of region information. The initial version which encodes regions from text description is shown in (a), and the current method which encodes background context is shown in (b).}
% \label{fig:exp_ablation}
% \end{figure}

\begin{figure}[ht]
\centering
\includegraphics[width=\linewidth]{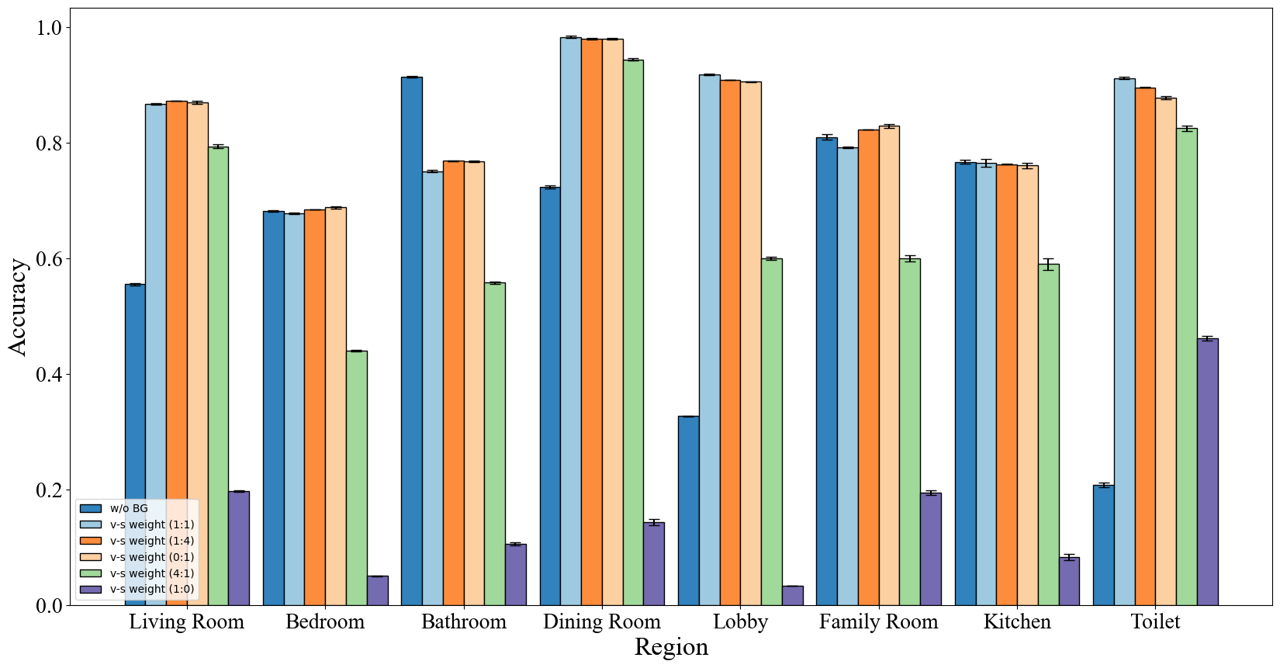}
\caption{Ablation results on the accuracy of region prediction on Matterport3D\cite{Matterport3D} with 3D positions input. The w/o BG stands for not encoding background pixels to get region embeddings, and v-s weight ablates the weight of vision-language and semantic embeddings in the embeddings similarity contribution. Error bars show the results among samples from different scenes in Matterport3D\cite{Matterport3D}.}
\label{fig:ablation2}
\end{figure}

\subsection{Hierarchical Approach Comparison}
Hierarchical scene representation is widely studied with numerous tasks, mainly employing scalable receptive fields and representations to fine-tune results of scalable objects and local relations. As Fig.\ref{comparing-hierarchical} shows, VoxFusion introduced octree map with various voxel sizes, LERF employed feature pyramids. As far as we know, few of them explicitly consider the layout level information and the association with objects and positions. This idea comes from recent neuroscience findings, and similar theory has not yet been introduced in scene representations.

\subsection{Topometric search for planning}
We employ a simple A* approach for planning. Given a topometric graph $G$, the start point $p$, and the target destination object text $t$. First, the belonged region $r$ of $p$ is inferred according to the main paper. The existing objects nodes embeddings are compared with the encoded visual-language and semantic embeddings of $t$ to find the target object node $o$. At the same time, if the region of destination object $r_d$ is declared, the search process would be more simple by directly search among region nodes. Here lists the pseudocode of the employed A*. 

\begin{algorithm}
\caption{AStar($G$, $r$, $o$)}
\begin{algorithmic}[1]
\State $openSet \gets \{r\}$ \Comment{Set of nodes to be evaluated}
\State $cameFrom \gets \{\}$ \Comment{Mapping of nodes to their parent nodes}
\State $gScore[r] \gets 0$ \Comment{Cost from start along best known path}
\State $fScore[r] \gets h(r, o)$ \Comment{Estimated total cost from start to goal}

\While{$openSet$ is not empty}
    \State $current \gets$ node in $openSet$ with lowest $fScore$ value
    \If{$current = o$}
        \State \Return ReconstructPath($cameFrom$, $o$)
    \EndIf
    \State remove $current$ from $openSet$
    
    \For{each neighbor $n$ of $current$}
        \State $tentativeGScore \gets gScore[current] + d(current, n)$
        \If{$tentativeGScore < gScore[n]$}
            \State $cameFrom[n] \gets current$
            \State $gScore[n] \gets tentativeGScore$
            \State $fScore[n] \gets gScore[n] + h(n, o)$
            \If{$n$ not in $openSet$}
                \State add $n$ to $openSet$
            \EndIf
        \EndIf
    \EndFor
\EndWhile

\State \Return "No path found"

\Function{ReconstructPath}{$cameFrom$, $current$}
    \State $path \gets [current]$
    \While{$current$ is in $cameFrom$}
        \State $current \gets cameFrom[current]$
        \State insert $current$ at the beginning of $path$
    \EndWhile
    \State \Return $path$
\EndFunction
\end{algorithmic}
\end{algorithm}

\subsection{Topometric map nodes examples}
We list the attributes of nodes and edges in the topometric map as example here in Listing $1-4$, including the object nodes, region nodes, and edges.

\begin{lstlisting}[language=python, caption=Region node]
{
    "id": 0,
    "node_type": region,
    "bbox_extent": [
        4.163309999999999,
        4.207343,
        2.53566175
    ],
    "bbox_center": [
        -8.821845,
        2.6915385,
        1.259409125
    ],
    "class": "bedroom",
    "caption": "A bedroom at the northwest of the house with warm lighting. Main objects include a bed in the center, a large closet, and a dresser at the corner."
},
\end{lstlisting}

\begin{lstlisting}[language=python, caption=Object node]
{
    "id": 1,
    "node_type": object,
    "bbox_extent": [
        0.3569,
        0.2297,
        0.101.8
    ],
    "bbox_center": [
        0.3222,
        -1.1108,
        -0.5062
    ],
    "class": "picture",
    "caption": "A white framed picture hanging on the wall."
},
\end{lstlisting}

\begin{lstlisting}[language=python, caption=Entrance node]
{
    "id": 0,
    "node_type": Entrance,
    "bbox_extent": [
        0.5,
        1.6,
        2.8,
    ],
    "bbox_center": [
        -3.244,
        -0.276,
        0.487
    ],
    "class": "Entrance",
    "caption": "Entrance connecting bedroom and living room."
},
\end{lstlisting}

\begin{lstlisting}[language=python, caption=Region entrance edge]
{
    "id": 2,
    "edge_type": region_entrance,
    "start_node": {
        "id": 0,
        "node_type": region,
        "bbox_extent": [
            4.163309999999999,
            4.207343,
            2.53566175
        ],
        "bbox_center": [
            -8.821845,
            2.6915385,
            1.259409125
        ],
        "region_tag": "bedroom"
    },
    "end_node": {
        "id": 0,
        "node_type": Entrance,
        "bbox_extent": [
            0.5,
            1.6,
            2.8,
        ],
        "bbox_center": [
            -3.244,
            -0.276,
            0.487
        ],
        "class": "Entrance",
        "caption": "Entrance connecting bedroom and living room."
    },
    "relationship": connected,
    "position_relation": "b to the southeast of a",
    "position_reason": "The x-coordinate of the center of bbox of end_node (-3.244) is larger than that of start_node (-8.821845), and the y-coordinates of the center of bbox of end_node (-0.276) is less than that of start_node (4.207343). Therefore, b is to the southeast of a."
    "caption": "The pathway from bedroom to living room."
},
\end{lstlisting}

\begin{lstlisting}[language=python, caption=Object region edge]
{
    "id": 2,
    "node_type": object_region,
    "start_node": {
        "id": 7,
        "node_type": object,
        "bbox_extent": [
            2.155,
            2.052,
            0.883
        ],
        "bbox_center": [
            5.598,
            2.566,
            0.136
        ],
        "class": "bed",
        "caption": "a bed with a white comforter and a pillow"
    },
    "end_node": {
        "id": 0,
        "node_type": region,
        "bbox_extent": [
            4.163309999999999,
            4.207343,
            2.53566175
        ],
        "bbox_center": [
            -8.821845,
            2.6915385,
            1.259409125
        ],
        "class": "bedroom"
        "caption": "A bedroom at the northwest of the house with warm lighting. Main objects include a bed in the center, a large closet, and a dresser at the corner."
    },
    "relationship": belong,
    "position_relation": "a in the center of b",
    "caption": "According to the bbox center position and extent, the bed is in the center of bedroom."
},
\end{lstlisting}

\subsection{Prompt Example for Region Node Connectivity Description}
With topometric mapped nodes, we leverage LLM to describe the connectivity of nodes according to the general knowledge and bounding box 3D position. In listing 5, here we provide a prompt example to describe the connectivity relationship between content objects and regions and set up the edge.

\begin{lstlisting}[caption=Prompt example to set up edge with nodes.]
{
DEFAULT_PROMPT_POST = """
You are an excellent graph managing agent. Given a graph nodes set of an environment,
you can explore the relationships of nodes with their attributes and build edges among
them.

The input is a list of JSONS describing two types of nodes, including the object and 
region. You need to produce a JSON string (and nothing else) and set up edges between them with keys: "relationship", "position_relation" and "caption".

Each of the JSON fields will have the following fields:
1. id: a unique number
2. node_type: type of this node
3. bbox_extent: the 3D bounding box extents
4. bbox_center: the 3D bounding box center
5. class: an extremely brief description
6. caption: a sentence describing node attributes in detail

Produce a "relationship" field that best describes the relationship of the object node and region node. Set "false" if the object is not related to the area or is not reasonable, the relationship is refused. Produce a
"position_relation" field describing the position relationship between object and region according to their
bounding box information in the 3D space. Before producing the "position_relation" field, produce a "caption" field that explains why the "position_relation" field is reasonable.

The built edges should include following fields:
1. id: a unique number of each edge in order
2. node_type: according to the connected node type in the form "start_node\_end_node"
3. start_node: keep JSON values of the object node unchanged
4. end_node: keep JSON values of the region node unchanged
5. relationship
6. position_relation
7. caption
"""
\end{lstlisting}

\subsection{Additional Experiment Results}
Additional experiments results of object localization using text query inputs and view localization using image query inputs. Also, a table is provided showing the metric on exactly each region class from 4 scenes in Matterport3D dataset.

\begin{table}[ht]
\label{exp_1}
\centering
\small
\setlength{\abovecaptionskip}{0.2cm}

\setlength{\tabcolsep}{3.2pt}
\begin{tabular}{ccccccccccccc}
\toprule % Top horizontal line
\multirow{2}{*}{\textbf{Regions}} & \multicolumn{3}{c}{\textbf{Scene1}} & \multicolumn{3}{c}{\textbf{Scene2}} & \multicolumn{3}{c}{\textbf{Scene3}} & \multicolumn{3}{c}{\textbf{Scene4}} \\ \cline{2-13}
                      & Acc.  & Pre.  & F1    & Acc.  & Pre.  & F1   & Acc.  & Pre.  & F1     & Acc.  & Pre.  & F1  \\ \hline
Living Room           & 0.948 & 0.970 & 0.959 & 0.870 & 0.881 & 0.875 & 0.778 & 0.810 & 0.793 & 0.902 & 0.949 & 0.925 \\
Bedroom               & 0.943 & 0.825 & 0.880 & 0.925 & 0.923 & 0.924 & 0.687 & 0.767 & 0.725 & 0.920 & 0.870 & 0.894 \\
% Utility Room          & 0.911 & 0.948 & 0.929 &   -   &   -   &   -   &   -   &   -   &   -   \\
Bathroom              & 0.466 & 0.680 & 0.554 & 0.903 & 0.898 & 0.901 & 0.875 & 0.463 & 0.605 & 0.797 & 0.831 & 0.814 \\
Dining Room           &   -   &   -   &   -   & 0.961 & 0.794 & 0.870 & 0.774 & 0.732 & 0.752 & 0.933 & 0.887 & 0.910 \\
Lobby                 & 0.681 & 0.941 & 0.790 & 0.853 & 0.951 & 0.899 & 0.978 & 0.510 & 0.671 & 0.855 & 0.698 & 0.769 \\
Family Room           &   -   &   -   &   -   &   -   &  - &  -   & 0.903 & 0.571 & 0.700 & 0.926 & 0.936 & 0.931 \\
Kitchen               & 0.994 & 0.654 & 0.789 & 0.788 & 0.836 & 0.811 & 0.833 & 0.833 & 0.833 & 0.758 & 0.854 & 0.803 \\
Office                &   -   &   -   &   -   & 0.969 & 0.848 & 0.905 &   -   &   -   &   -   & 0.953 & 0.883 & 0.917 \\
Toilet                &   -   &   -   &   -   &   -   &   -   &   -   & 0.900 & 0.711 & 0.795 &   -   &   -   &   -   \\ 
\midrule % In-table horizontal line
\midrule % In-table horizontal line
{\footnotesize Avg. Acc./Samples}   & \multicolumn{3}{c}{0.886 / 169k} & \multicolumn{3}{c}{0.900 / 185k} & \multicolumn{3}{c}{0.884 / 111k} & \multicolumn{3}{c}{0.894 / 112k} \\
\bottomrule % Bottom horizontal line
\end{tabular}
\caption{Region prediction results on the test set of different scenes from the Matterport3D\cite{Matterport3D} dataset. Accuracy, precision, and F1 score are used as metrics.}
\end{table}

\begin{figure}[ht]
\label{comparing-hierarchical}
\centering
\includegraphics[width=0.7\linewidth]{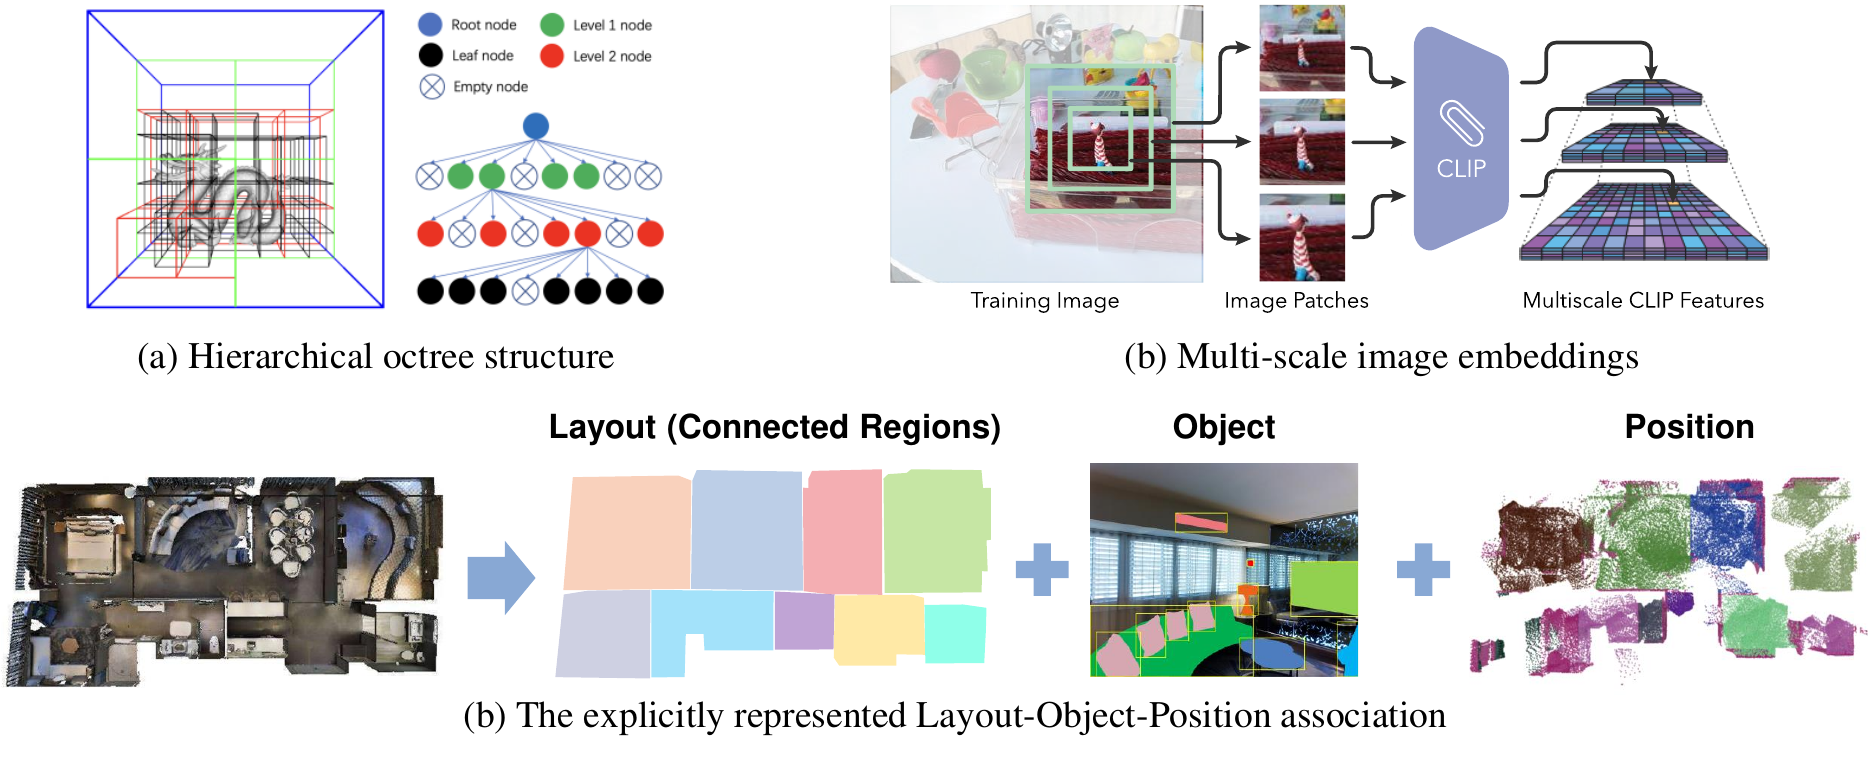}
\vspace{-0.15in}
\caption{The comparison of the hierarchical scene representation strategy against previous works.}
\vspace{-0.3in}
\end{figure}

\begin{figure}[h]
\centering
\includegraphics[width=.91\linewidth]{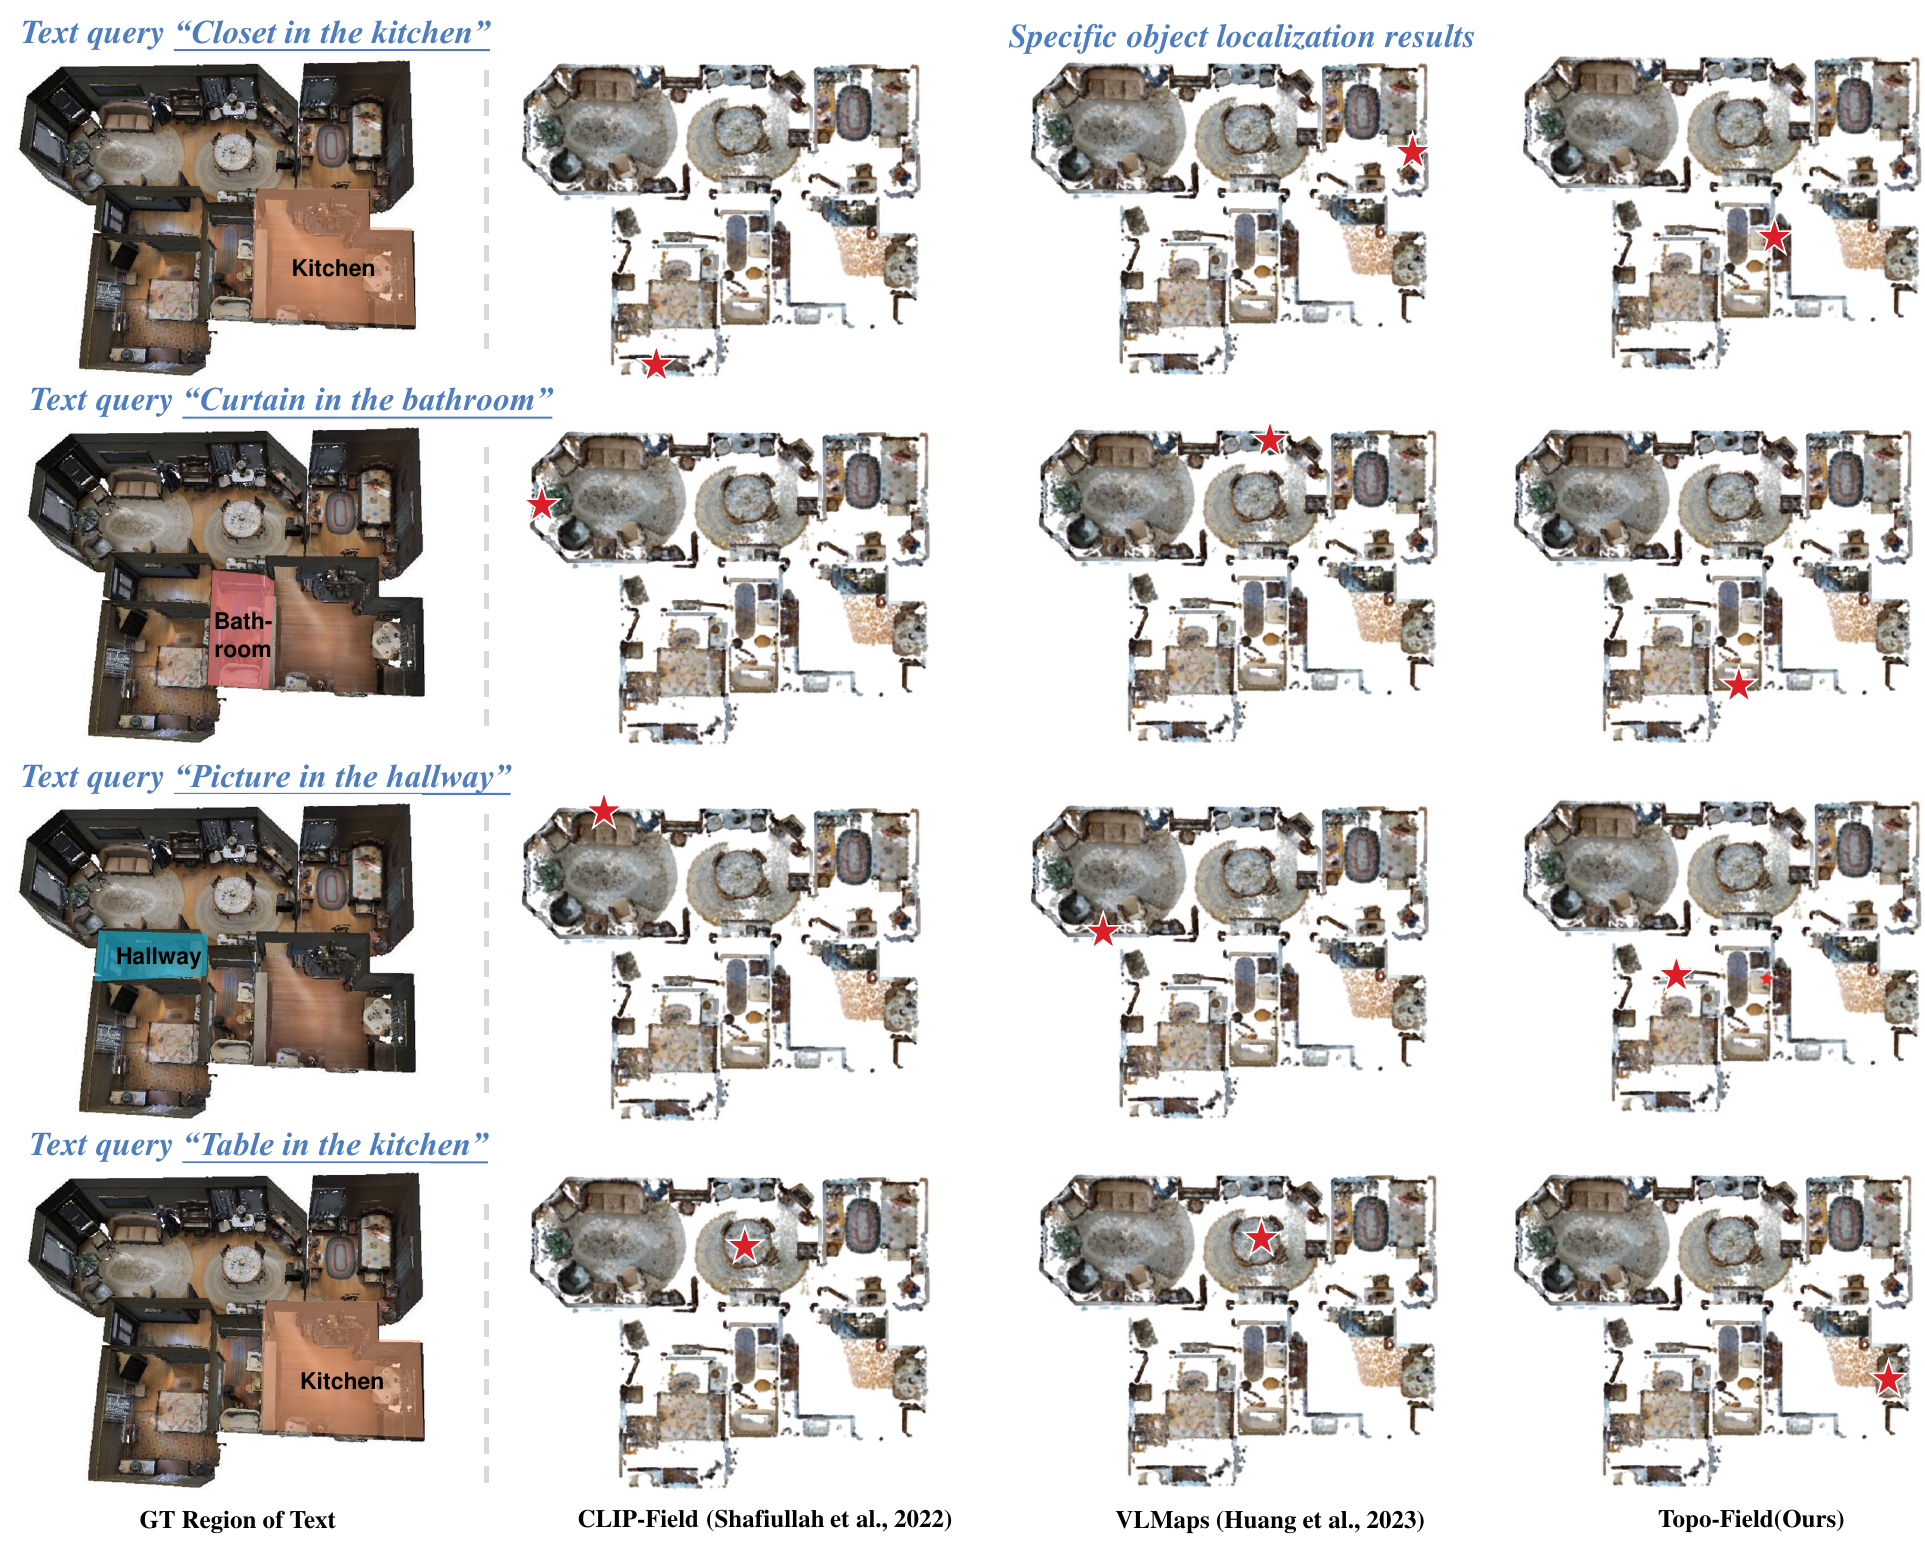}
\caption{Text query localization on scene 2t7WUuJeko7\cite{Matterport3D}.}
\end{figure}

\begin{figure}[h]
\centering
\includegraphics[width=.91\linewidth]{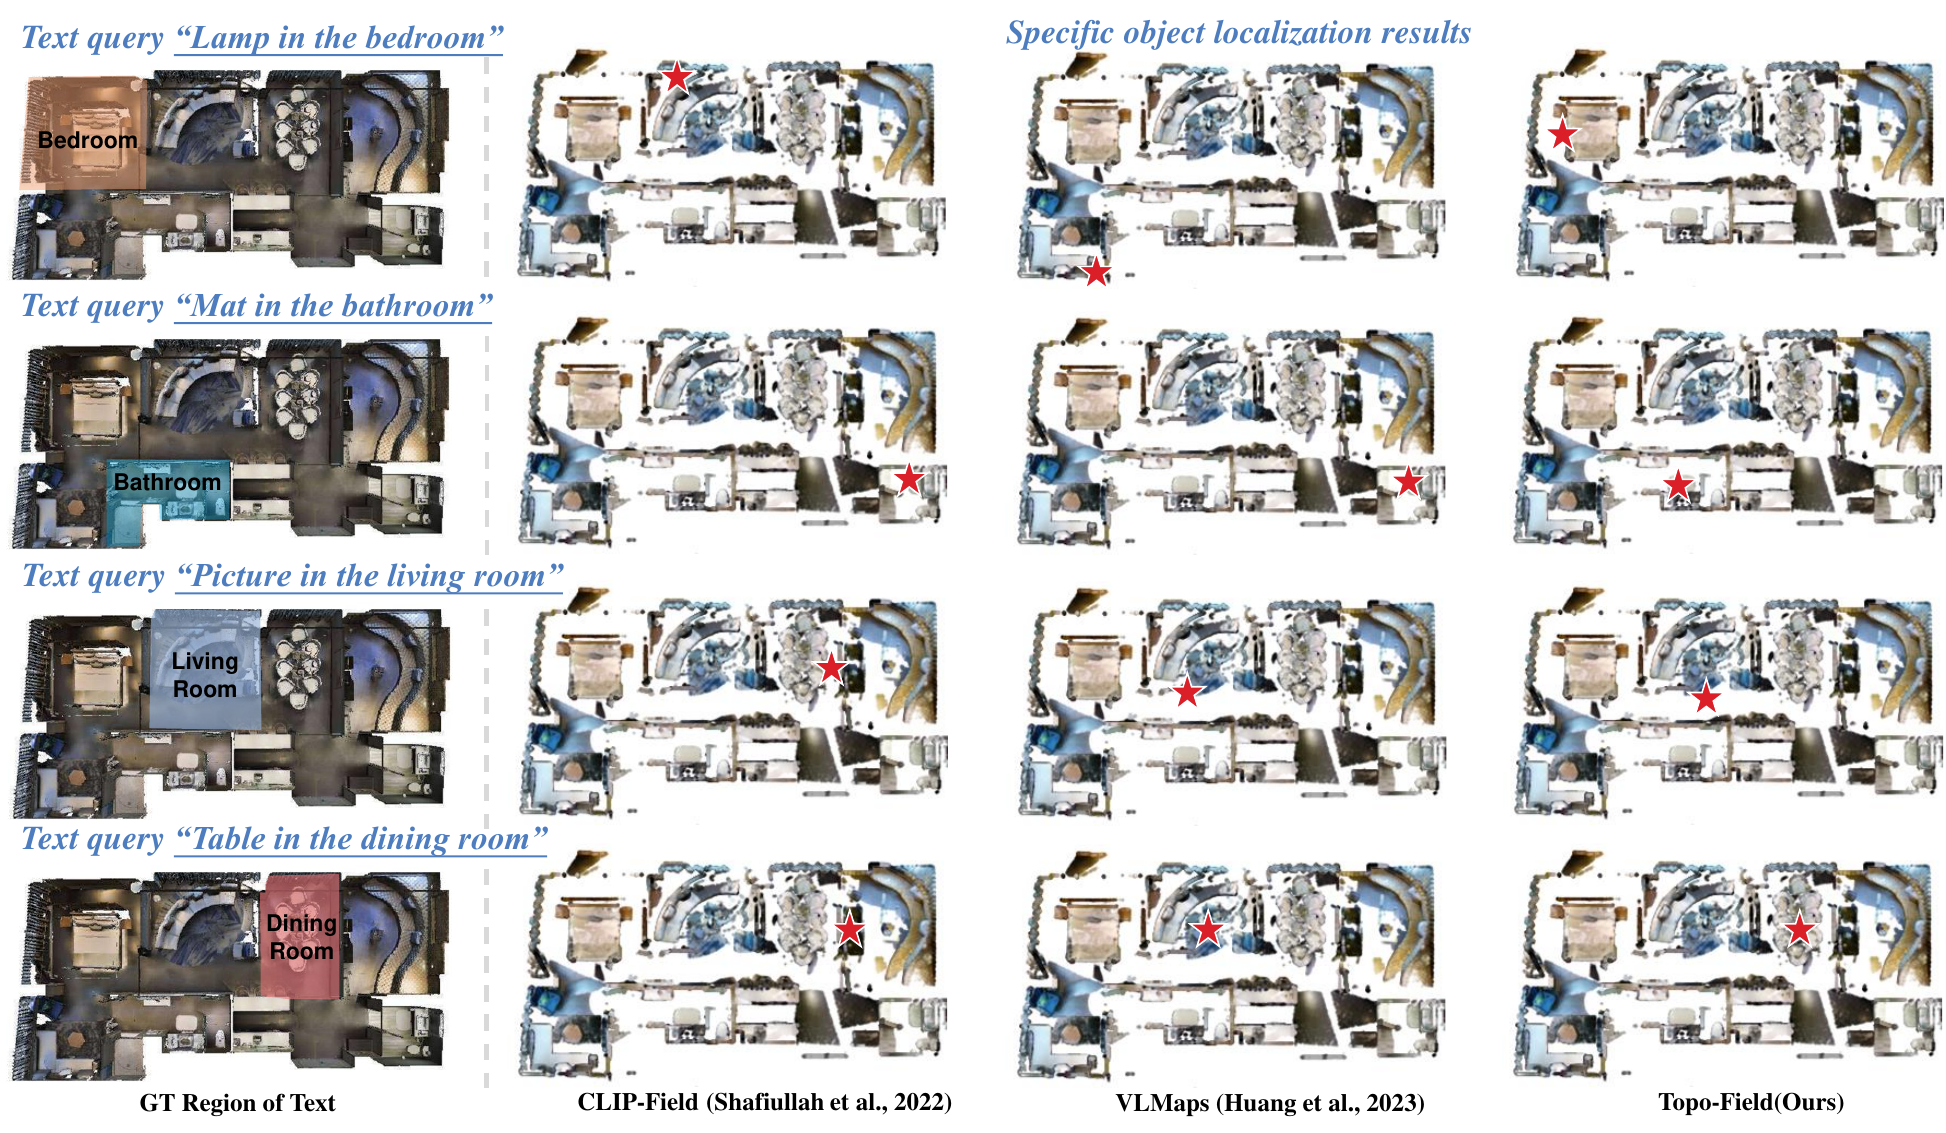}
\caption{Text query localization on scene 17DRP5sb8fy\cite{Matterport3D}.}
% \label{fig:exp3}
\end{figure}

\begin{figure}[h]
\centering
\includegraphics[width=.91\linewidth]{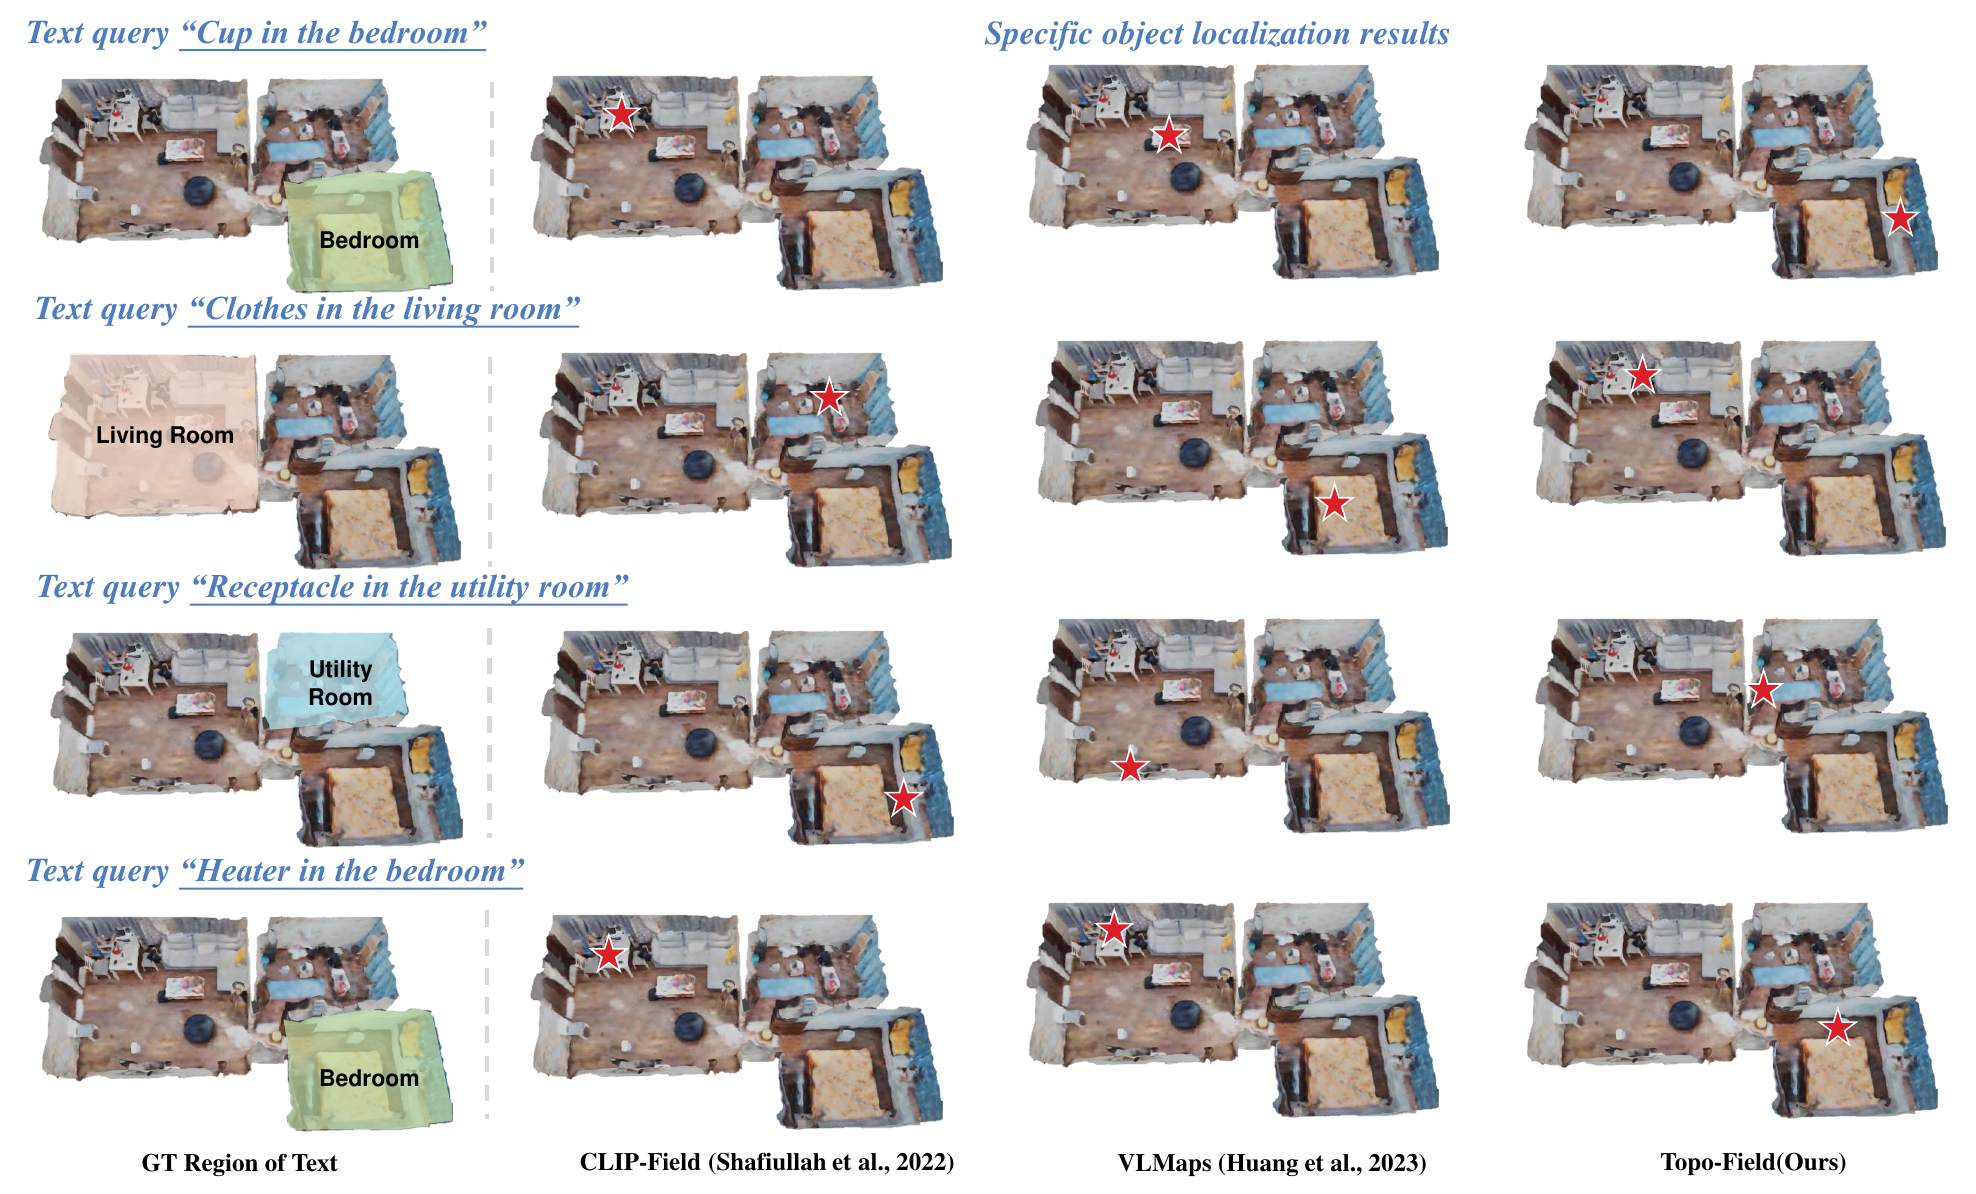}
\caption{Text query localization on scene Apartment\cite{niceslam}.}
% \label{fig:exp3}
\end{figure}

\begin{figure}[h]
\centering
\includegraphics[width=.91\linewidth]{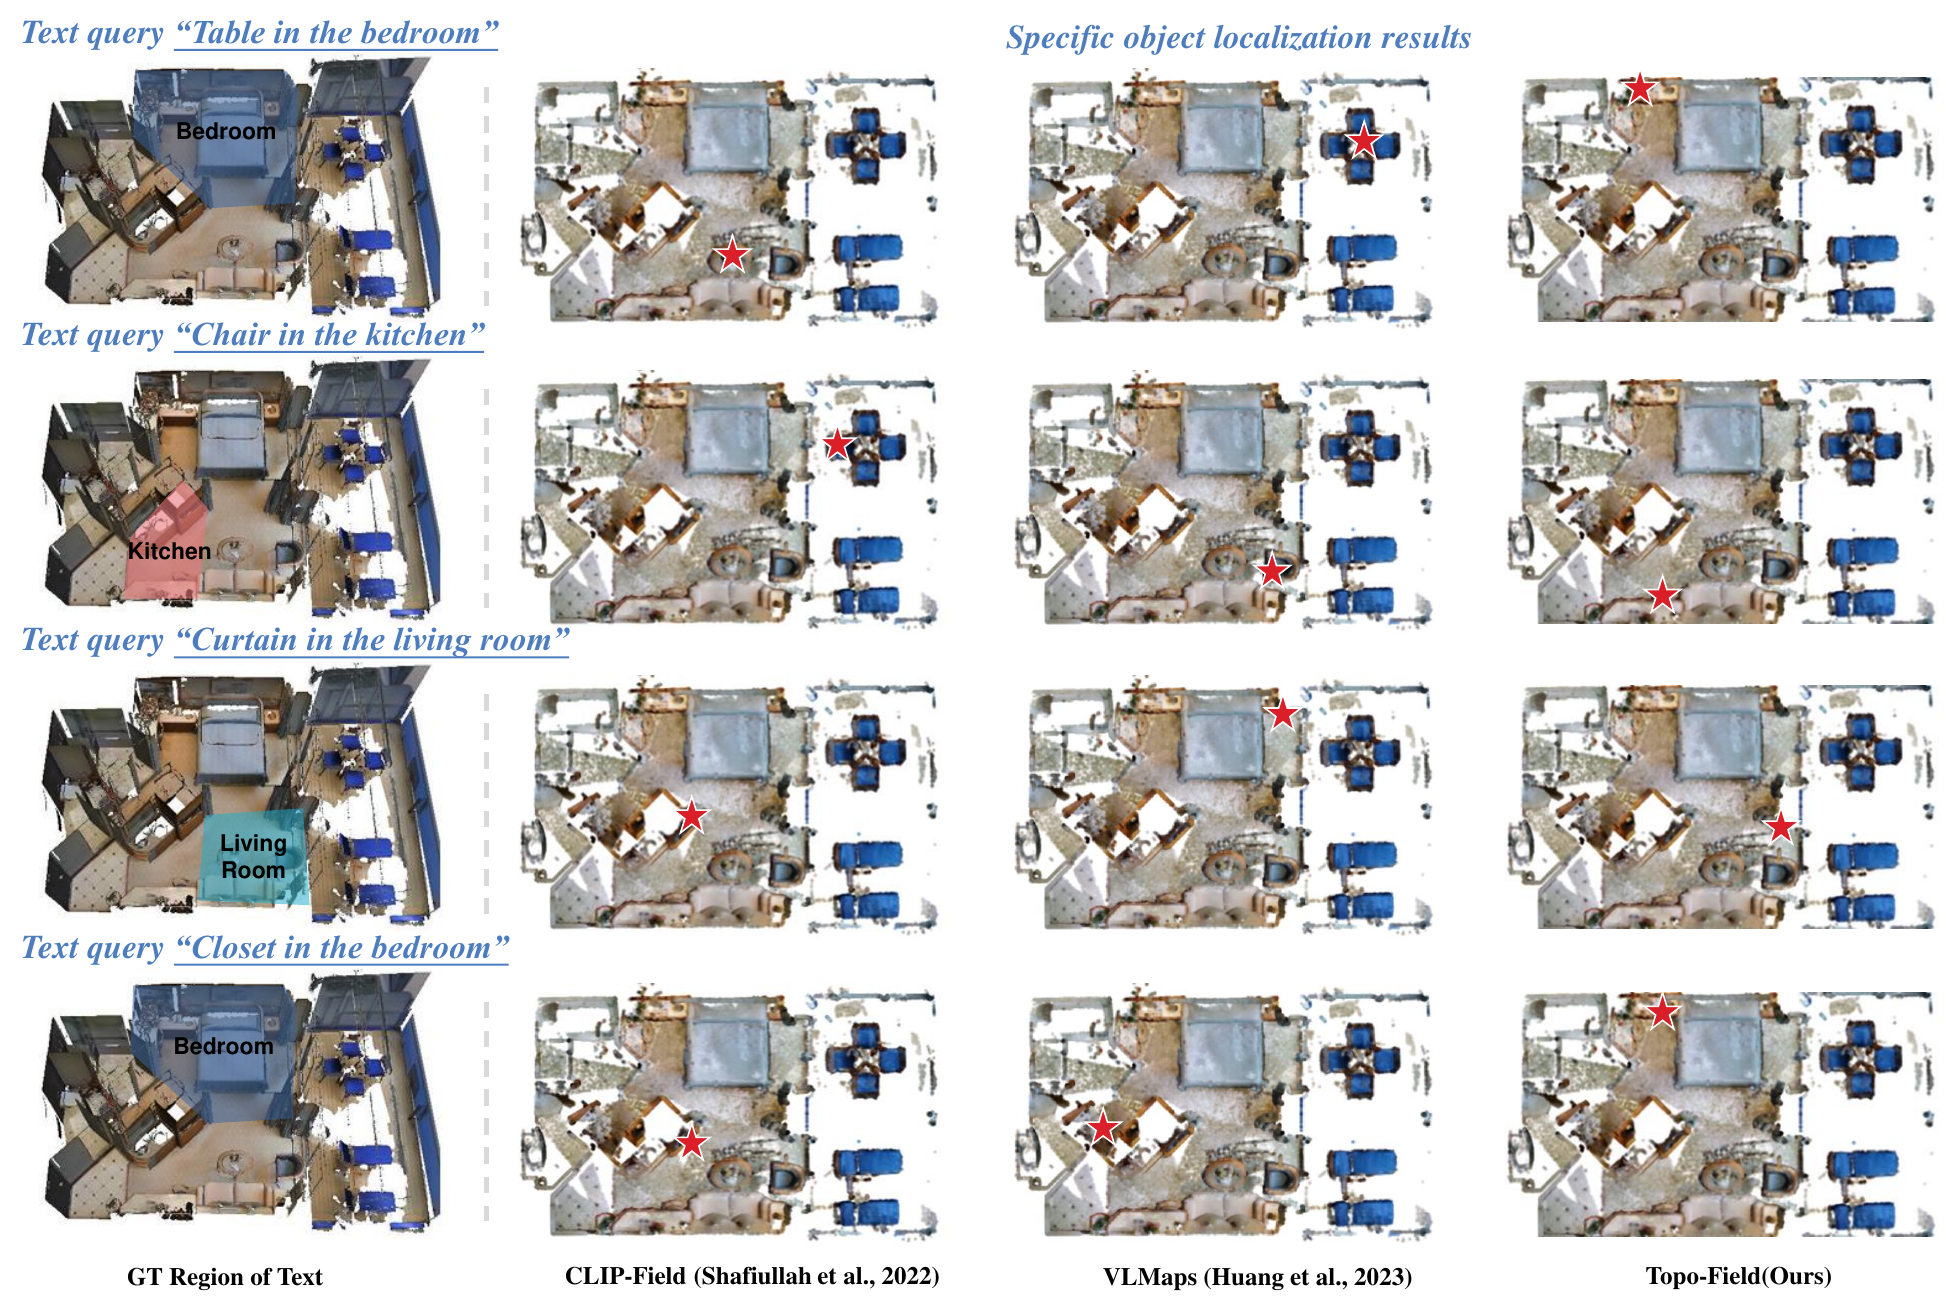}
\caption{Text query localization on scene HxpKQynjfin\cite{Matterport3D}.}
% \label{fig:exp3}
\end{figure}

\begin{figure}[h]
\centering
\includegraphics[width=.91\linewidth]{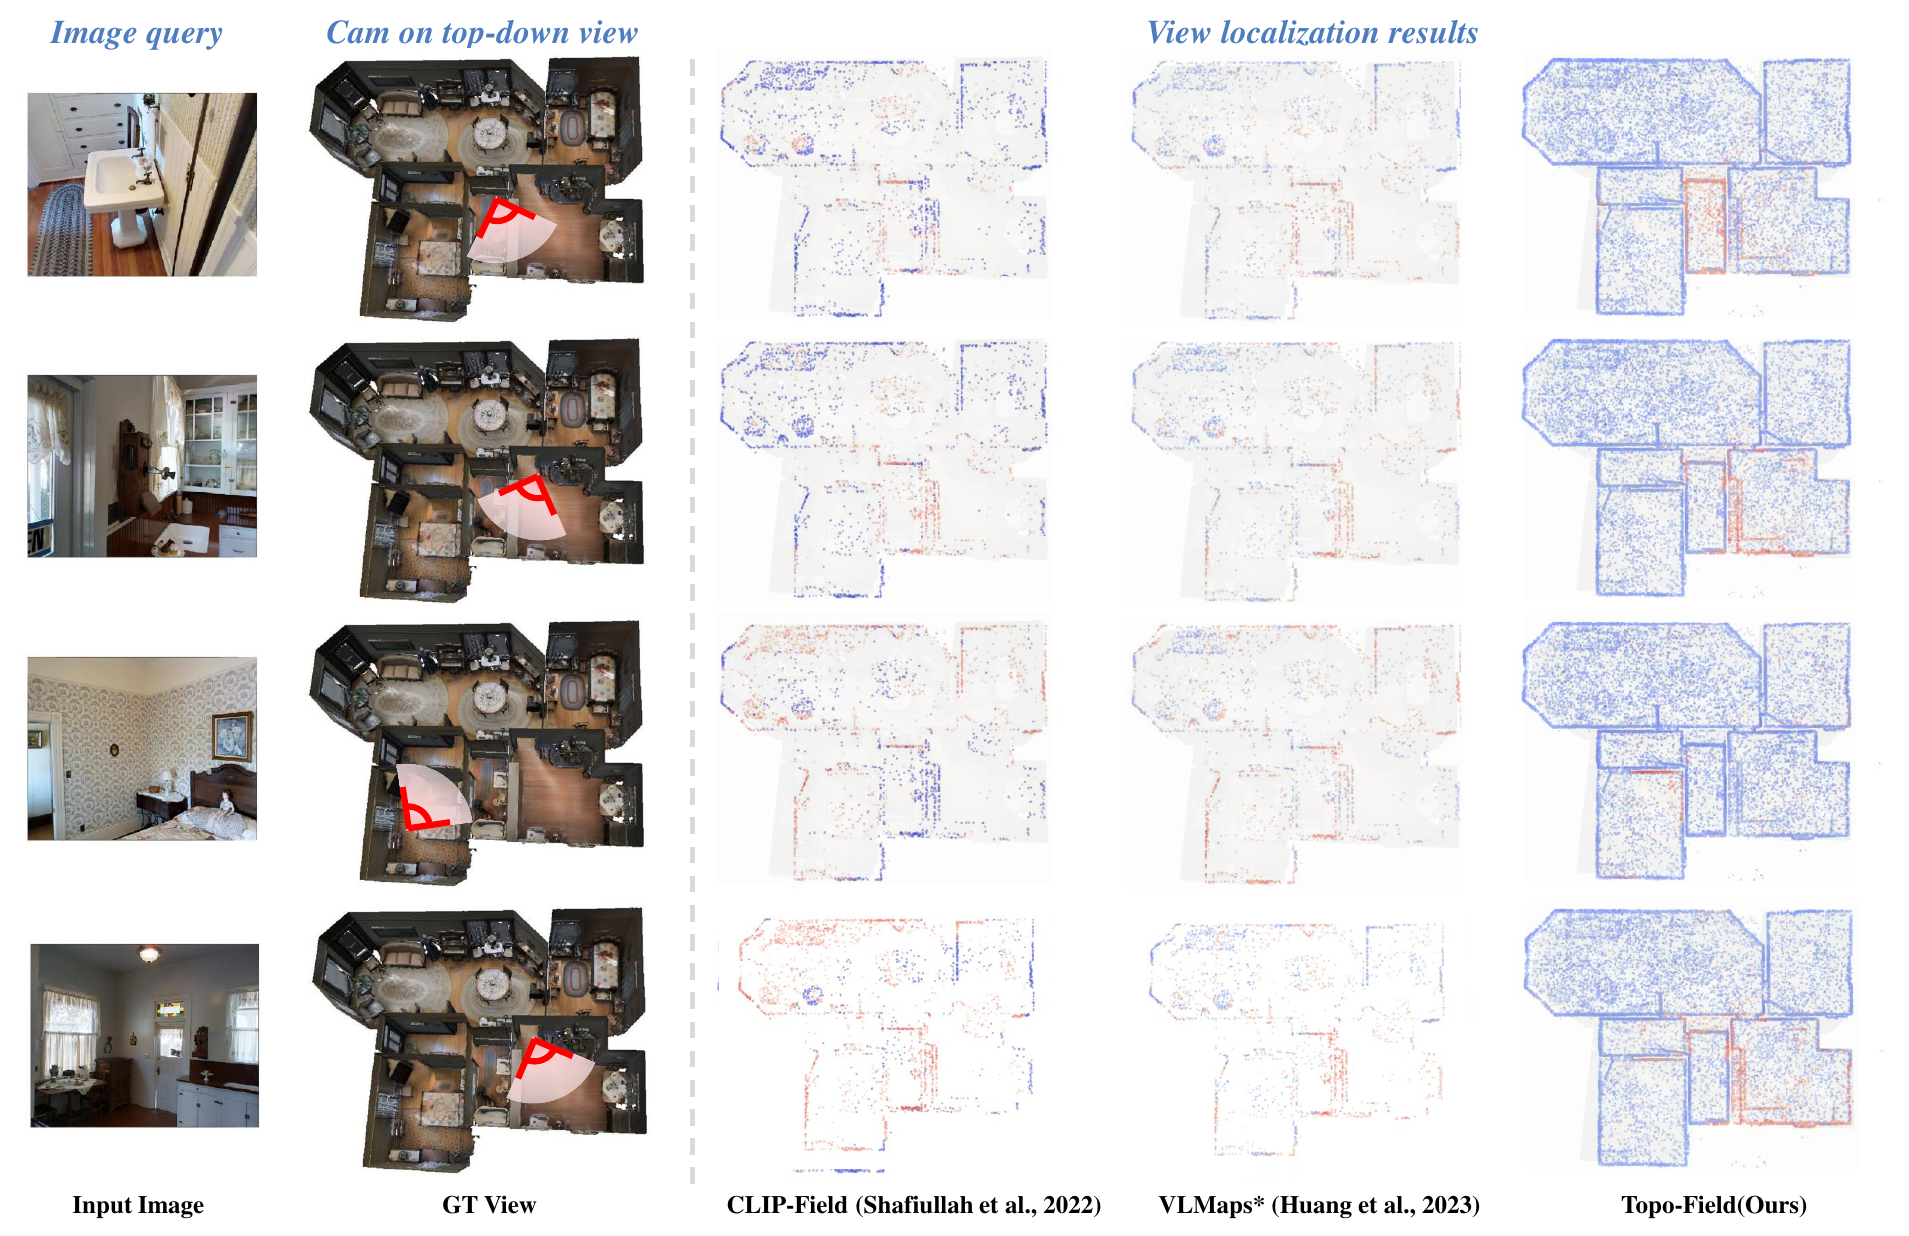}
\caption{Image query localization on scene 2t7WUuJeko7\cite{Matterport3D}.}
\end{figure}

\begin{figure}[h]
\centering
\includegraphics[width=.91\linewidth]{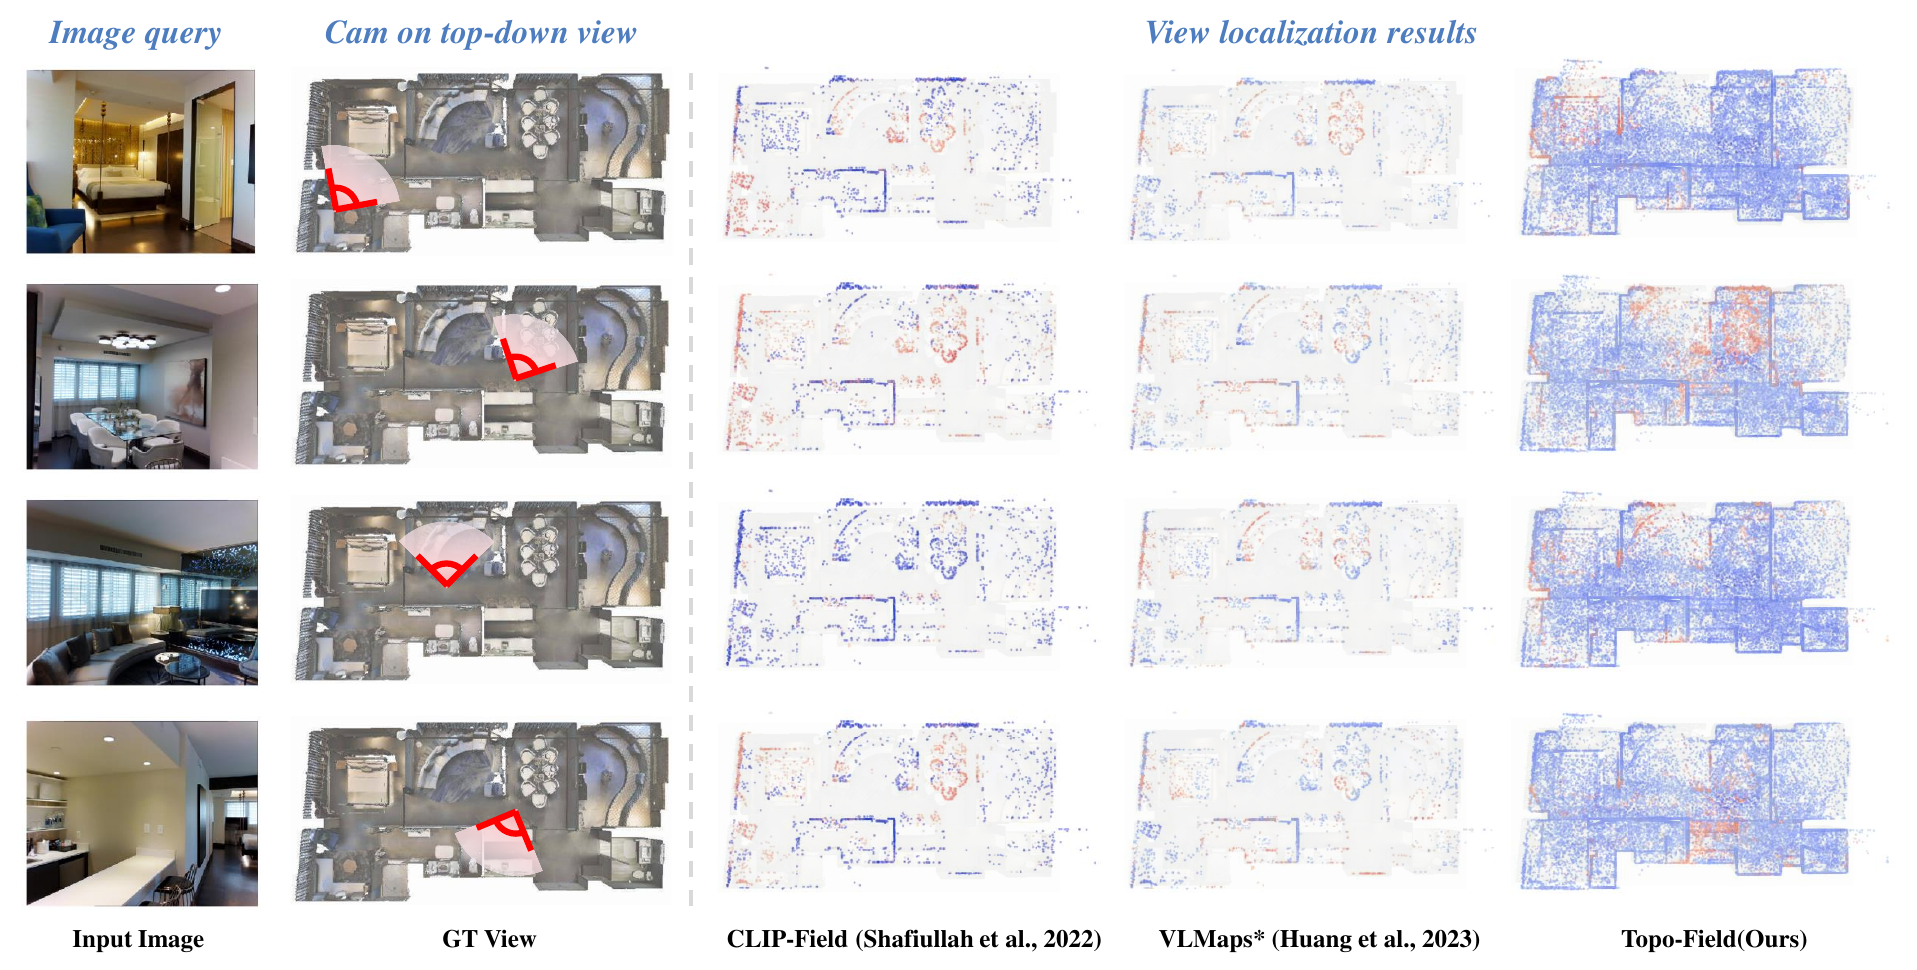}
\caption{Image query localization on scene 17DRP5sb8fy\cite{Matterport3D}.}
% \label{fig:exp3}
\end{figure}

\begin{figure}[h]
\centering
\includegraphics[width=.91\linewidth]{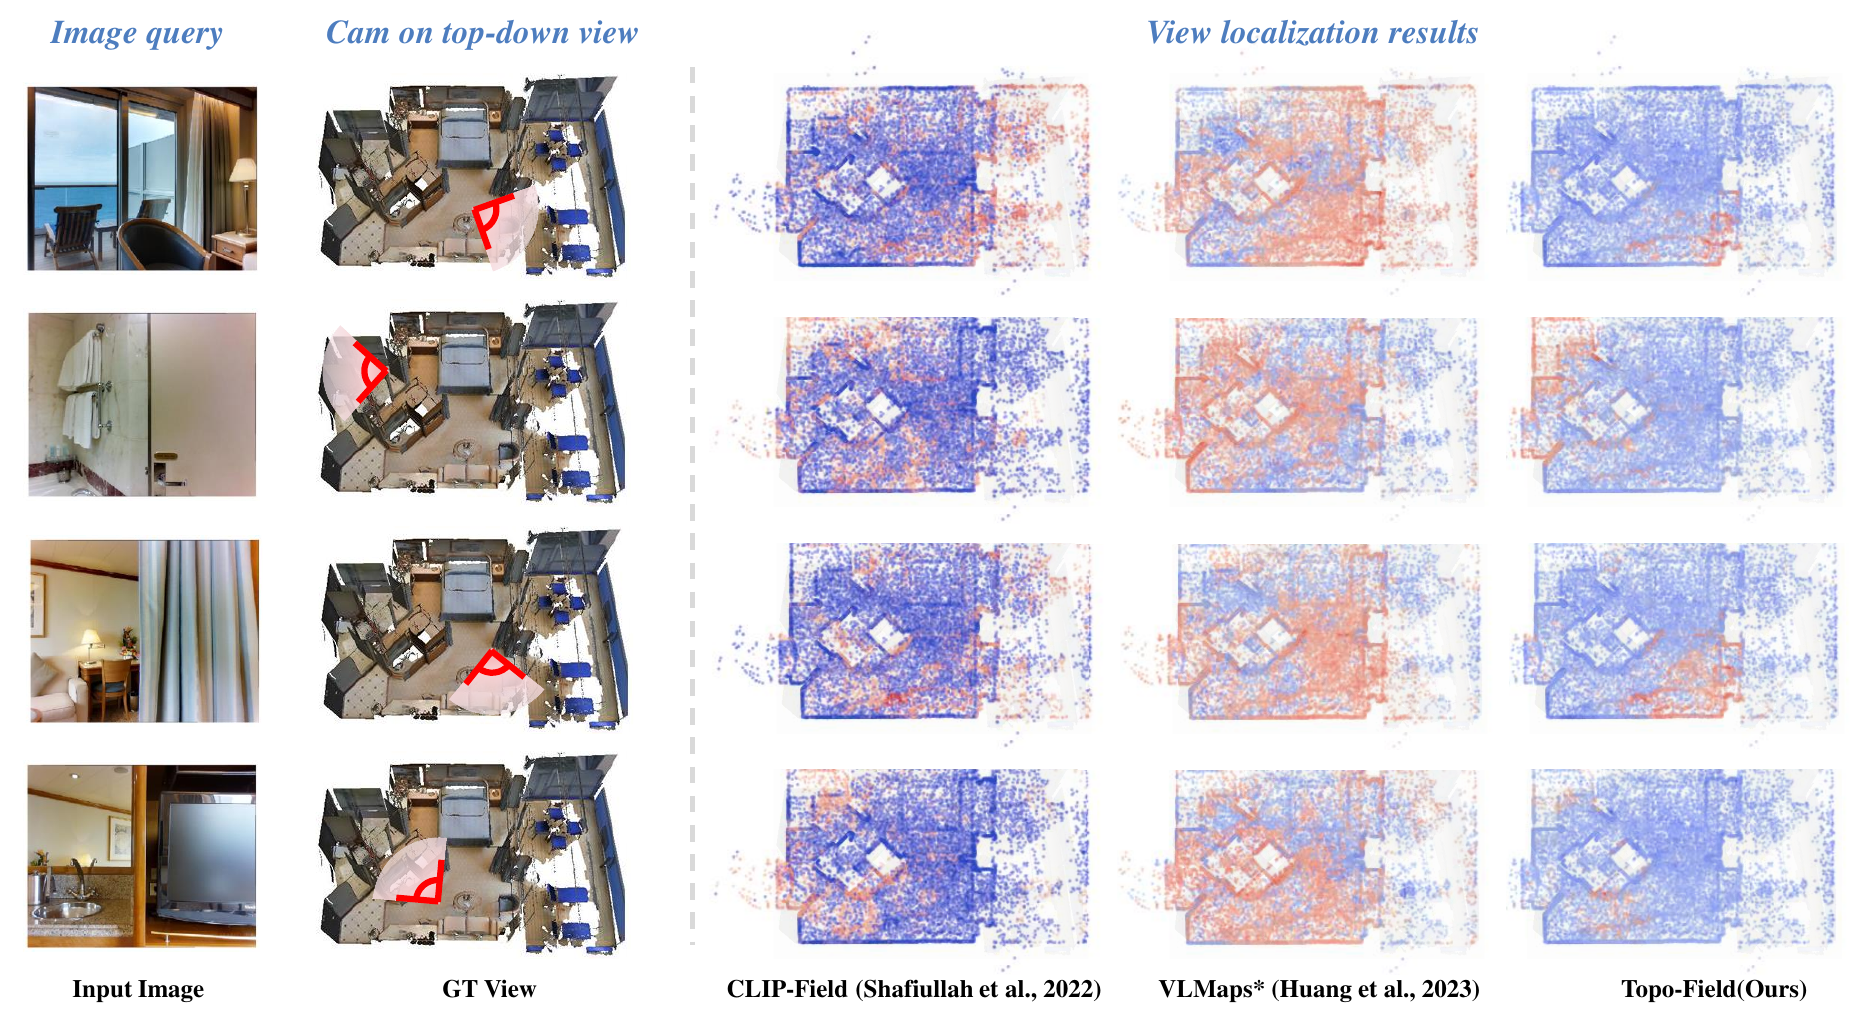}
\caption{Image query localization on scene HxpKQynjfin\cite{Matterport3D}.}
% \label{fig:exp3}
\end{figure}
